# Supplementary material for: Finite-Size Spectral Signatures of Order by Quantum Disorder: A Perspective from Anderson's Tower of States
Source: arXiv:2509.10610 source file (2026-04-10)
Supplement: Supplementary file 1 [file supp.pdf]

# Supplemental Material for “Finite-Size Spectral Signatures of Order by Quantum Disorder: A Perspective from Anderson’s Tower of States”

Subhankar Khatua,<sup>1,2,3</sup> Griffin C. Howson,<sup>1,2</sup> Michel J. P. Gingras,<sup>1,4</sup> and Jeffrey G. Rau<sup>2</sup>

<sup>1</sup>Department of Physics and Astronomy, University of Waterloo, Waterloo, Ontario, N2L 3G1, Canada

<sup>2</sup>Department of Physics, University of Windsor, 401 Sunset Avenue, Windsor, Ontario, N9B 3P4, Canada

<sup>3</sup>Institute for Theoretical Solid State Physics, IFW Dresden and Würzburg-Dresden

Cluster of Excellence ct.qmat, Helmholtzstr. 20, 01069 Dresden, Germany

<sup>4</sup>Waterloo Institute for Nanotechnology, University of Waterloo, Waterloo, Ontario, N2L 3G1, Canada

(Dated: September 12, 2025)

## I. EFFECTIVE LIEB-MATTIS MODEL

To understand the mechanism of order by quantum disorder (ObQD) in a quantum spin-1/2 system, we develop an effective theory based on the Lieb-Mattis (LM) description which has previously been employed to investigate the finite-size signatures of spontaneous symmetry breaking [1–3]. The LM Hamiltonian can be obtained by projecting the full spin Hamiltonian onto its low-energy subspace [4, 5],  $P\mathcal{H}P \equiv \mathcal{H}_{\text{LM}}$ , where  $P$  is the projector onto the subspace. This subspace can be determined by identifying the classical ordering pattern of the system’s ground state or alternatively through the spin-spin correlation functions of the quantum ground state obtained via exact diagonalization (ED). For example, if the classical ground state ordering is ferromagnetic, the relevant subspace is the ‘ferromagnetic’ Hilbert space of total spin  $S_{\text{tot}} = N/2$  where  $N$  is the total number of  $S = 1/2$  spins. Here, the projected Hamiltonian would involve a single “large” spin  $S_{\text{tot}}$  of length  $N/2$ , which can be solved exactly. For more complex orders involving multiple sublattices  $N_s$ , the projection needs to be onto the subspace of  $N_s$  large spins, each of length  $\tilde{N}/2$ , where  $\tilde{N} = N/N_s$  is the number of spins in each sublattice. Ref. [4] outlines a straightforward way to perform these projections, making use of the fact that the projected Hamiltonian must be symmetric under any permutation of spins within a sublattice. To illustrate this procedure, consider a Hamiltonian term of the form,  $S_{\mathbf{r}}^{\mu} S_{\mathbf{r}'}^{\nu}$  where  $\mathbf{r}, \mathbf{r}'$  are lattice sites and  $\mu, \nu = x, y, z$  denote components. The projection of this term can be achieved as follows –

*Different sublattices.*— If  $\mathbf{r}$  and  $\mathbf{r}'$  belong to two different sublattices, say,  $A$  and  $B$  respectively,

$$PS_{\mathbf{r}}^{\mu} S_{\mathbf{r}'}^{\nu} P = \frac{S_A^{\mu} S_B^{\nu}}{\tilde{N}^2}, \quad (\text{S1})$$

where  $S_A^{\mu}$  and  $S_B^{\nu}$  are each of spin-length  $\tilde{N}/2$ .

*Same sublattice.*— To obtain the projection when  $\mathbf{r}$  and  $\mathbf{r}'$  belong to the same sublattice, e.g.,  $A$ , we start from the relation

$$\begin{aligned} S_{A,\text{tot}}^{\mu} S_{A,\text{tot}}^{\nu} &= \sum_{\mathbf{r} \in A} S_{\mathbf{r}}^{\mu} S_{\mathbf{r}}^{\nu} + \sum_{\mathbf{r} \neq \mathbf{r}' \in A} S_{\mathbf{r}}^{\mu} S_{\mathbf{r}'}^{\nu} \\ &= \frac{\tilde{N}\delta_{\mu\nu}}{4} I + \frac{i\epsilon_{\mu\nu\sigma}}{2} S_{A,\text{tot}}^{\sigma} + \sum_{\mathbf{r} \neq \mathbf{r}' \in A} S_{\mathbf{r}}^{\mu} S_{\mathbf{r}'}^{\nu}, \quad (\text{S2}) \end{aligned}$$

where  $S_{A,\text{tot}} = \sum_{\mathbf{r} \in A} S_{\mathbf{r}}$ . In the last step in Eq. (S2), we have made use of the algebra of Pauli matrices and  $I$  is an identity matrix. From Eq. (S2), using spin permutation symmetry

within this sublattice, we obtain

$$PS_{\mathbf{r}}^{\mu} S_{\mathbf{r}'}^{\nu} P = \frac{1}{\tilde{N}(\tilde{N}-1)} \left( S_A^{\mu} S_A^{\nu} - \frac{\tilde{N}\delta_{\mu\nu}}{4} I - \frac{i\epsilon_{\mu\nu\sigma}}{2} S_A^{\sigma} \right), \quad (\text{S3})$$

where again  $S_A^{\mu}$  is an emergent spin of length  $\tilde{N}/2$ . The denominator  $\tilde{N}(\tilde{N}-1)$  arises from projecting the last term in Eq. (S2) which sums over all spin-spin interaction pairs within sublattice- $A$  considering double counting, with  $(\tilde{N}-1)$  pairs for each spin.

Eqs. (S1) and (S3) provide the necessary projections to derive the LM Hamiltonian, corresponding to the full microscopic Hamiltonian. A similar description may also be obtained using a semiclassical approach based on the spin path integral formalism [6–9].

## II. HEISENBERG-COMPASS MODEL ON THE SQUARE LATTICE

### A. Ferromagnetic regime

*Derivation of the Lieb-Mattis Hamiltonian.*— Here, we elaborate on the formalism for constructing the LM Hamiltonian of the Heisenberg compass model on the square-lattice. Although the Hamiltonian has already been introduced in the main text, we provide it again here for the convenience of discussion. The Hamiltonian is given by

$$\mathcal{H} = \sum_{\mathbf{r}} \left[ J \sum_{\delta=\mathbf{x},\mathbf{y}} S_{\mathbf{r}} \cdot S_{\mathbf{r}+\delta} + K \left( S_{\mathbf{r}}^x S_{\mathbf{r}+\mathbf{x}}^x + S_{\mathbf{r}}^y S_{\mathbf{r}+\mathbf{y}}^y \right) \right], \quad (\text{S4})$$

where  $S_{\mathbf{r}}$  represents a spin-1/2 operator at site  $\mathbf{r}$  on the square lattice and  $\delta = \mathbf{x}, \mathbf{y}$  refers to the nearest-neighbor bonds. We parametrize  $J \equiv \cos \xi$  and  $K \equiv \sin \xi$  with  $\pi < \xi < 3\pi/2$ , such that both couplings are ferromagnetic (i.e., negative). As discussed in the main text, the classical ground states are uniform fully polarized ferromagnetic configurations along arbitrary directions in the  $\hat{\mathbf{x}} - \hat{\mathbf{y}}$  plane, given by

$$S_{\mathbf{r}} = S (\cos \phi \hat{\mathbf{x}} + \sin \phi \hat{\mathbf{y}}), \quad (\text{S5})$$

where  $\phi \in [0, 2\pi)$  characterizes the orientation of the magnetization relative to the  $\hat{\mathbf{x}}$  axis. Since the classical ground states are ferromagnetic, i.e., has one magnetic sublattice, as discussed in Sec. I, the relevant low-energy subspace is the space of  $S_{\text{tot}} = N/2$ . Thus, to construct the LM Hamiltonian of this

model, we project the Hamiltonian in Eq. (S4) onto the sector  $S_{\text{tot}} = N/2$ . Using Eq. (S3), we have

$$PS_r^\mu S_{r'}^\mu P = \frac{(S_{\text{tot}}^\mu)^2 - \frac{N}{4}I}{N(N-1)}, \quad (\text{S6})$$

and finally the LM Hamiltonian of Eq. (S4) is:

$$\begin{aligned} \mathcal{H}_{\text{LM}} &= \frac{2J[S_{\text{tot}}^2 - \frac{3N}{4}I] + K[(S_{\text{tot}}^x)^2 + (S_{\text{tot}}^y)^2 - \frac{N}{2}I]}{N-1} \\ &= \frac{2J[S_{\text{tot}}^2 - \frac{3N}{4}I] + K[(S_{\text{tot}}^2 - (S_{\text{tot}}^z)^2 - \frac{N}{2}I)]}{N-1}. \end{aligned} \quad (\text{S7})$$

In the sector  $S_{\text{tot}} = N/2$ ,  $S_{\text{tot}}^2$  is proportional to the identity operator. Ignoring all terms that are proportional to the identity operator, we have

$$\mathcal{H}_{\text{LM}} = -\frac{K}{(N-1)}(S_{\text{tot}}^z)^2. \quad (\text{S8})$$

This describes a planar rotor. Its spectrum is discussed in the main text and begins to capture some qualitative features of the ED data [see the main text for more details]. We reiterate here that this Hamiltonian has a U(1) symmetry, a consequence of the classical accidental degeneracy of the parent Hamiltonian [Eq. (S4)], and thus, does not exhibit ObQD. We must go beyond the LM description to be able to capture ObQD.

*Derivation of the Beyond Lieb-Mattis Hamiltonian.*— As discussed in the main text, to investigate the effects of ObQD, we add an additional term to the LM Hamiltonian [Eq. (S8)] corresponding to the spin-wave zero-point energy (ZPE). The ZPE in this model is of the form  $-g \cos(4\phi)$  [10] where,  $g$  denotes the ObQD energy scale. We will now rewrite this term in such a way that can be easily promoted to the operator form in the  $S_{\text{tot}} = N/2$  subspace. The components of the total spin in the classical ground states are  $S_{\text{tot}}^x = \frac{N}{2} \cos \phi$  and  $S_{\text{tot}}^y = \frac{N}{2} \sin \phi$ , giving  $S_{\text{tot}}^+ \equiv (S_{\text{tot}}^x + i S_{\text{tot}}^y) = \frac{N}{2} \exp(i\phi)$  and  $S_{\text{tot}}^- \equiv (S_{\text{tot}}^x - i S_{\text{tot}}^y) = \frac{N}{2} \exp(-i\phi)$ . Thus, in terms of the total classical spin, the ZPE may be written as

$$-g \cos(4\phi) = -\frac{g}{2} \frac{(S_{\text{tot}}^+)^4 + (S_{\text{tot}}^-)^4}{(N/2)^4}. \quad (\text{S9})$$

Therefore, the minimal term that needs to be added to Eq. (S8) to take into account ObQD is the operator equivalent of Eq. (S9), which is

$$-\frac{g}{2} \frac{(S_{\text{tot}}^+)^4 + (S_{\text{tot}}^-)^4}{[N/2(N/2+1)]^2}, \quad (\text{S10})$$

where  $S_{\text{tot}}^+$  refers to the raising operator in the  $S_{\text{tot}} = N/2$  subspace and we have modified  $(N/2)^2 \rightarrow N/2(N/2+1)$  to account for the classical to quantum spin-length conversion. Note that this replacement is a phenomenological or ad hoc normalization. The precise  $N$ -dependence could in principle be derived from higher-order many-body perturbation theory. However, this is computationally challenging for anisotropic

Hamiltonians [11]. Nevertheless, the qualitative physics remains unaffected by the exact normalization. In our phenomenological effective description, we adopt  $N/2(N/2+1)$  to reflect naturally the quantum analog of spin-length of the effective large spin. With this, the beyond Lieb-Mattis (BLM) model of the ferromagnetic Heisenberg-compass model on the square lattice is given by

$$\mathcal{H}_{\text{BLM}} = \mathcal{H}_{\text{LM}} - \frac{g}{2} \frac{(S_{\text{tot}}^+)^4 + (S_{\text{tot}}^-)^4}{[N/2(N/2+1)]^2}. \quad (\text{S11})$$

Note that ZPE is an extensive quantity (i.e.,  $\propto N$ ), thus  $g \propto N$ . Thus, for a  $4 \times 4$  square lattice,  $g$  is quite small and therefore, the additional term in Eq. (S11) behaves as a perturbation to the bare LM Hamiltonian, modifying the bare spectrum of Eq. (S8) slightly. Identifying

$$\mathcal{H}_{\text{pert}} \equiv -\frac{g}{2} \frac{(S_{\text{tot}}^+)^4 + (S_{\text{tot}}^-)^4}{[N/2(N/2+1)]^2}, \quad (\text{S12})$$

this perturbation will split the degenerate  $m = \pm 2$  states of the bare LM Hamiltonian at the first order. To see this explicitly, we construct the perturbation matrix on the  $m = \pm 2$  space

$$\mathbf{W} \equiv \begin{bmatrix} \langle -2|\mathcal{H}_{\text{pert}}| - 2 \rangle & \langle -2|\mathcal{H}_{\text{pert}}| + 2 \rangle \\ \langle +2|\mathcal{H}_{\text{pert}}| - 2 \rangle & \langle +2|\mathcal{H}_{\text{pert}}| + 2 \rangle \end{bmatrix}, \quad (\text{S13})$$

where the diagonal terms are zero as can be seen from the form of the perturbation. The off-diagonal term is given by

$$\begin{aligned} \langle -2|\mathcal{H}_{\text{pert}}| + 2 \rangle &= -\frac{g \langle -2|[(S_{\text{tot}}^+)^4 + (S_{\text{tot}}^-)^4]| + 2 \rangle}{2[N/2(N/2+1)]^2} \\ &= -\frac{g \langle -2|(S_{\text{tot}}^-)^4| + 2 \rangle}{2[N/2(N/2+1)]^2} \\ &= -\frac{g(N/2-1)(N/2+2)}{N(N/2+1)}, \end{aligned} \quad (\text{S14})$$

and  $\langle +2|\mathcal{H}_{\text{pert}}| - 2 \rangle = \langle -2|\mathcal{H}_{\text{pert}}| + 2 \rangle = -\frac{g(N/2-1)(N/2+2)}{N(N/2+1)}$ . The eigenvalues of  $\mathbf{W}$  are  $\pm \frac{g(N/2-1)(N/2+2)}{N(N/2+1)}$  and thus, the splitting of the  $m = \pm 2$  states under the perturbation  $\mathcal{H}_{\text{pert}}$  is  $\Delta = \frac{2g(N/2-1)(N/2+2)}{N(N/2+1)}$ . We equate this  $\Delta$  with the splitting observed in ED to get an estimate of the ObQD energy scale  $g$  from ED. That is, we take

$$g = \frac{N/2(N/2+1)}{(N/2-1)(N/2+2)} \Delta_{\text{ED}}, \quad (\text{S15})$$

where  $\Delta_{\text{ED}}$  is the splitting obtained from ED. A comparison of  $g$  obtained from ED to that obtained from LSWT on the  $N$ -site square-lattice is provided in the main text.

## B. Antiferromagnetic regime

We extend our study of the Heisenberg-compass model on the square lattice to the antiferromagnetic regime ( $0 < \xi < \pi/2$ ) where  $J > 0, K > 0$ . The classical ground states in this

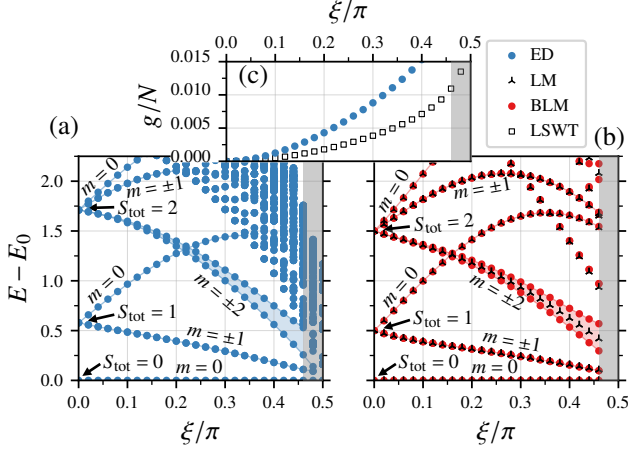

FIG. S1. Antiferromagnetic Heisenberg-compass model on the square lattice of  $N = 16$  sites with periodic boundary conditions. (a) Low-energy ED spectrum. (b) Spectrum of the corresponding LM and BLM models. The value of  $g$  in the BLM model is extracted from the splitting in the ED spectrum. (c) Comparison of  $g$  obtained from LSWT and ED spectrum. Grey areas in all panels mark the regime where the low-energy physics deviates from the BLM picture because of a new state appearing in the microscopic model at  $\xi = \pi/2$  [10].

regime are accidentally degenerate Néel states with arbitrary Néel-vector orientation in the  $\hat{x} - \hat{y}$  plane [10], described by

$$\mathbf{S}_r = (-1)^r S (\cos \phi \hat{x} + \sin \phi \hat{y}), \quad (\text{S16})$$

where  $\phi \in [0, 2\pi)$  characterizes the orientation of the staggered magnetization relative to the  $\hat{x}$  axis. Similar to the ferromagnetic regime, the accidentally degenerate ground states form an  $O(2)$  manifold. The occurrence of ObQD in this regime has been demonstrated in Ref. [10] using spin-wave theory, which selects the Néel states along  $\pm\hat{x}, \pm\hat{y}$  directions.

To probe the signatures of ObQD in this antiferromagnetic regime in the spin-1/2 limit, we perform ED exploiting the same symmetry (i.e., discrete translation symmetry of the model) as done in the ferromagnetic regime. The resulting ED spectrum is shown in Fig. S1(a). To identify which features in this spectrum arise from ObQD, we follow the same effective BLM model construction as introduced for the ferromagnetic regime. To this end, we first derive the corresponding LM Hamiltonian. Unlike the ferromagnetic ground states in the ferromagnetic regime, here we have Néel states—two sublattices ( $A$  and  $B$ ) in the unit cell. Thus, as explained in Sec. I, the LM model comes from projecting the full Hamiltonian onto the subspace formed by two large spins  $S_A = \tilde{N}/2 = N/4$  and  $S_B = N/4$ . Using Eq. (S1) on Eq. (S4), we have

$$\begin{aligned} \mathcal{H}_{\text{LM}} &= \frac{8JS_A \cdot S_B + 4K(S_A^x S_B^x + S_A^y S_B^y)}{N} \\ &= \frac{4J + 2K}{N}(S_{\text{tot}}^2 - S_A^2 - S_B^2) - \frac{4K}{N}S_A^z S_B^z, \end{aligned} \quad (\text{S17})$$

where  $S_{\text{tot}} \equiv S_A + S_B$  (sum of two  $N/4$ -length spins). For this  $\mathcal{H}_{\text{LM}}$ , while  $S_{\text{tot}}$  is not a good quantum number,  $S_{\text{tot}}^z$

is. Fig. S1(b) shows the LM spectrum with  $m$  denoting the eigenvalues of  $S_{\text{tot}}^z$ . At  $\xi = 0$ , the model reduces to the isotropic Heisenberg antiferromagnet (HAF) on the square lattice which enjoys a true  $SU(2)$  symmetry, and thus  $S_{\text{tot}}$  is conserved too, labeled in Fig. S1(b). As  $\xi$  is varied from zero to introduce finite compass interactions, the  $m = 0$  state [adiabatically connected to  $S_{\text{tot}} = 1$ ] and  $m = \pm 2$  states [connected to  $S_{\text{tot}} = 2$ ] cross at  $\xi \sim 0.16\pi$  without mixing due to their distinct  $m$  values. The LM spectrum shows good qualitative agreement with the low-energy ED spectrum of the full Hamiltonian, as displayed in Fig. S1(a). However, the splitting of  $m = \pm 2$  states observed in the ED spectrum is *absent* in the LM spectrum. This has to do with the  $U(1)$  symmetry of  $\mathcal{H}_{\text{LM}}$ , reflecting the accidental degeneracy in the ground states—thus failing to capture ObQD.

As in the case of the ferromagnetic regime [Sec. II A],  $\mathcal{H}_{\text{LM}}$  must be augmented by the operator corresponding to the spin-wave ZPE to obtain the BLM Hamiltonian. The ZPE takes the form  $-g \cos(4\phi)$  with four minima [ $\phi = 0, \pi/2, \pi, 3\pi/2$ ] corresponding to the four Néel configurations along the  $\pm\hat{x}, \pm\hat{y}$  directions [10]. The components of the staggered magnetization in the ground states,  $n_{\text{tot}}^x = S_A^x - S_B^x = \frac{N}{2} \cos \phi$  and  $n_{\text{tot}}^y = S_A^y - S_B^y = \frac{N}{2} \sin \phi$ , giving  $n_{\text{tot}}^+ \equiv (n_{\text{tot}}^x + in_{\text{tot}}^y) = \frac{N}{2} \exp(i\phi)$  and  $n_{\text{tot}}^- \equiv (n_{\text{tot}}^x - in_{\text{tot}}^y) = \frac{N}{2} \exp(-i\phi)$ . Thus, in terms of the staggered magnetization, the ZPE is  $-(g/2)[(n_{\text{tot}}^+)^4 + (n_{\text{tot}}^-)^4]/(N/2)^4$ . Therefore, the minimal term that needs to be added to Eq. (S17) to take into account ObQD is

$$-\frac{g}{2} \frac{[(n_{\text{tot}}^+)^4 + (n_{\text{tot}}^-)^4]}{2^4 \left[\frac{N}{4}(\frac{N}{4} + 1)\right]^2}, \quad (\text{S18})$$

where we have shifted  $(N/4)^2 \rightarrow (N/4)(N/4 + 1)$  to account for the conversion of classical to quantum spin-length corresponding to each sublattice  $A$  and  $B$ . Thus, the BLM model for the antiferromagnetic Heisenberg-compass model on the square lattice is given by

$$\mathcal{H}_{\text{BLM}} \equiv \mathcal{H}_{\text{LM}} - \frac{g}{2} \frac{(S_A^+ - S_B^+)^4 + (S_A^- - S_B^-)^4}{[N/2(N/2 + 2)]^2}, \quad (\text{S19})$$

This added term behaves as a perturbation on  $\mathcal{H}_{\text{LM}}$  since  $g$  is weaker for smaller systems. First-order in this perturbation changes  $S_A^z$  and  $S_B^z$  in such a way that the states satisfying  $\Delta m = \pm 4$  split, thus we expect splitting of the  $m = \pm 2$  level. To extract the  $g$  value from the splitting of the  $m = \pm 2$  in the ED spectrum, we compute the first-order perturbation splitting within the BLM description numerically with  $g$  as an undetermined multiplicative parameter, and then equate it to the splitting in ED. We find an overall good agreement between the BLM and ED spectra using this extracted value, as shown in Fig. S1(b). Fig. S1(c) shows a comparison of the  $g$  obtained from LSWT and from the splitting of  $m = \pm 2$  states in the ED spectrum, differing only roughly by a factor of two.

### III. HEISENBERG-KITAEV MODEL ON THE HONEYCOMB LATTICE

#### A. Antiferromagnetic regime

Heisenberg-Kitaev model on the honeycomb lattice in the antiferromagnetic regime has been discussed in the main text. Here, we provide the details of the derivations of the corresponding LM and BLM Hamiltonians. The model is described by the Hamiltonian

$$\mathcal{H} = \sum_{\langle rr' \rangle_\gamma} [JS_r \cdot S_{r'} + KS_r^\gamma S_{r'}^\gamma], \quad (\text{S20})$$

where  $J, K$  are the Heisenberg and Kitaev couplings, respectively, and  $\gamma = x, y, z$  refer to both spin components and the three distinct nearest-neighbor bonds. This model possesses discrete rotation symmetries like  $C_3$  about the axis perpendicular to the lattice plane,  $C_2$  about the bond directions, and spin-only  $C_2$  rotations about  $\hat{x}, \hat{y}, \hat{z}$  directions. We take  $J \equiv \cos \xi$  and  $K \equiv \sin \xi$  with  $0 < \xi < \pi/2$ , such that both couplings are antiferromagnetic. As discussed in the main text, the classical ground states are accidentally degenerate Néel states with Néel vector oriented along any arbitrary direction and ObQD selects only those along the cubic axes (i.e.,  $\pm \hat{x}, \pm \hat{y}, \pm \hat{z}$ ) [12–14]. Since the classical ground state is a Néel order, the LM Hamiltonian can be obtained by projecting Eq. (S20) onto the subspace spanned by two spins  $S_A$  and  $S_B$  of length  $N/4$ , exactly as done for the antiferromagnetic Heisenberg-compass model in Sec. II B. Using the projection in Eq. (S1) on the full Hamiltonian [Eq. (S20)], we obtain

$$\mathcal{H}_{\text{LM}} = \frac{3J + K}{N} (S_{\text{tot}}^2 - S_A^2 - S_B^2). \quad (\text{S21})$$

In this case, the LM Hamiltonian exhibits an augmented SU(2) symmetry, thus resulting in both  $S_{\text{tot}}$  and  $S_{\text{tot}}^z$  as good quantum numbers. The spectrum of Eq. (S21) is discussed in the main text.

To include ObQD in the effective description, the LM Hamiltonian needs to be augmented by the operator equivalent of the spin-wave ZPE. The ZPE minimizes for the Néel states with Néel-vector along the cubic axes [12–14], taking the form of the cubic anisotropy on the ground state manifold. This can be written as an operator in the two-spin subspace as

$$-g \frac{[(S_A^x - S_B^x)^4 + (S_A^y - S_B^y)^4 + (S_A^z - S_B^z)^4]}{[N/4(N/4 + 1)]^2}. \quad (\text{S22})$$

This cubic anisotropy term breaks the SU(2) symmetry of  $\mathcal{H}_{\text{LM}}$ , which was accidental for the full model [Eq. (S20)], and restores all the discrete symmetries as mentioned above. For smaller systems, this term acts as a perturbation on  $\mathcal{H}_{\text{LM}}$ , analogous to the cubic crystal electric field effect on a SU(2) symmetric magnetic single ion. This splits the  $S_{\text{tot}} = 2$  and higher energy levels of  $\mathcal{H}_{\text{LM}}$ . The level  $S_{\text{tot}} = 2$  splits into the spin-analog of an orbital  $e_g$  doublet and  $t_{2g}$  triplet [15]. This splitting is also observed in the ED spectrum. To determine  $g$  from this splitting in ED, we numerically find the

first-order perturbation splitting of  $S_{\text{tot}} = 2$  states within BLM picture due to the perturbation in Eq. (S22) with  $g$  as an undetermined multiplicative factor and equate this splitting to that from ED. The comparison of  $g$  obtained from the splitting in ED spectrum and LSWT has been presented in the main text.

In principle, one can further understand the splitting of the  $S_{\text{tot}} = 3$  level within this description. However, these states are difficult to identify in ED spectrum due to level crossings with high energy non-rotor states which intrude above the  $S_{\text{tot}} = 2$  level.

#### B. Ferromagnetic regime

We move on now to consider the ferromagnetic regime with  $\pi < \xi < 3\pi/2$  such that  $J < 0, K < 0$ . In contrast to the antiferromagnetic regime, the classical ground states in this regime are fully polarized ferromagnetic states pointing along any arbitrary direction, with ObQD selecting only those aligned along the cubic axes (i.e.,  $\pm \hat{x}, \pm \hat{y}, \pm \hat{z}$ ), as shown using spin-wave theory [12–14]. We next perform ED, and the resulting spectrum is shown in Fig. S2(a). To identify the characteristic splittings induced by ObQD in the ED spectrum, we construct the corresponding BLM Hamiltonian, following the same approach as in the previous examples. Since the classical ground state manifold is ferromagnetic, the projection involved in the effective description needs to be done on the space of single spin of length  $S_{\text{tot}} = N/2$ , as done previously for the ferromagnetic Heisenberg-compass model on the square lattice. Making use of the projections derived for the ferromagnetic Heisenberg-compass model [Eq. (S6)] and omitting additive constants, we obtain

$$\mathcal{H}_{\text{LM}} = \frac{3J + K}{2(N - 1)} S_{\text{tot}}^2. \quad (\text{S23})$$

As in the antiferromagnetic regime, the LM Hamiltonian exhibits an enhanced SU(2) symmetry, meaning both  $S_{\text{tot}}$  and  $S_{\text{tot}}^z$  are good quantum numbers. All the different  $S_{\text{tot}}^z$  states within the  $S_{\text{tot}} = N/2$  subspace are degenerate. Consequently, the LM model energy eigenvalues, when shifted by the ground state energy  $E_0$ , are all zero, i.e.,  $E - E_0 = 0$  for each  $\xi$ . For this reason, we do not show the LM spectrum in Fig. S2.

To break the SU(2) symmetry of the LM Hamiltonian down to the discrete symmetries of the full model, we next consider the spin-wave ZPE. This ZPE acts as a cubic anisotropy on the classical ground state manifold [12–14], yielding the following operator in the  $S_{\text{tot}} = N/2$  space

$$-g \frac{(S_{\text{tot}}^x)^4 + (S_{\text{tot}}^y)^4 + (S_{\text{tot}}^z)^4}{(N/2(N/2 + 1))^2}. \quad (\text{S24})$$

This poses a cubic crystal field problem on the  $S_{\text{tot}} = N/2$  manifold rather than on the  $S_{\text{tot}} = 2$  manifold in the antiferromagnetic regime. To estimate  $g$  from ED, we use the splitting marked in light blue in the ED spectrum in Fig. S2(a). We numerically find the first-order perturbation (corresponding) splitting within the BLM model with  $g$  as an undetermined multiplicative parameter and equate it to the splitting in the



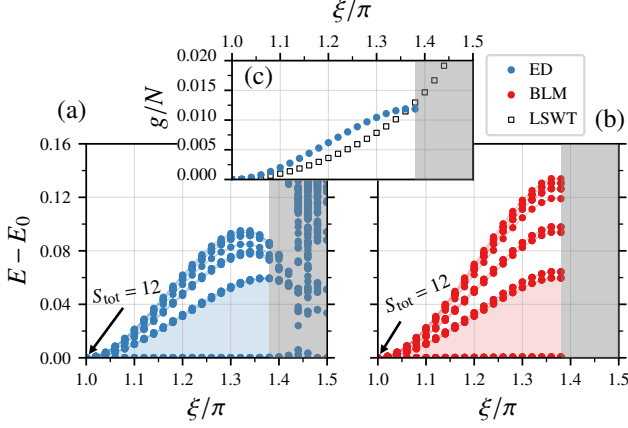

FIG. S2. Ferromagnetic Heisenberg-Kitaev model on the honeycomb lattice of  $N = 24$  sites with periodic boundary conditions. (a) Low-energy ED spectrum. (b) BLM model spectrum. The  $g$  value in BLM description is determined from the splitting in the ED spectrum. (c)  $g$  obtained from LSWT and ED spectrum. Grey areas in all panels mark the regime where the low-energy physics deviates from the BLM description.

ED spectrum, yielding an estimate for  $g$  from ED. Upon numerically diagonalizing the BLM Hamiltonian with these values of  $g$ , we observe that the cubic anisotropy term lifts the degeneracy of the  $S_{\text{tot}} = N/2$  multiplet, as seen in the BLM spectrum in Fig. S2(b), following the same degeneracy pattern of the split states in the ED spectrum [Fig. S2(a)]. We note good agreement between  $g$  obtained from ED and that obtained from LSWT, depicted in Fig. S2(c). However, this agreement breaks down in the range  $1.38\pi \lesssim \xi \lesssim 1.5\pi$  (grey shaded region in Fig. S2), possibly due to the onset of Kitaev spin liquid physics around  $\xi \sim 3\pi/2$ , where the BLM description is no longer valid.

#### IV. HEISENBERG-KITAEV MODEL ON THE CHAIN

To round out our discussion of two- and three-dimensional systems explored in the main text, we present here results for a one-dimensional version of the ferromagnetic Heisenberg-Kitaev model, namely, the Heisenberg-Kitaev spin chain, known for its potential in providing insights into two-dimensional Kitaev physics [16–19]. It is governed by the Hamiltonian

$$\mathcal{H} = J \sum_{i=1}^N \mathbf{S}_i \cdot \mathbf{S}_{i+1} + K \sum_i^{N/2} (S_{2i-1}^x S_{2i}^x + S_{2i}^y S_{2i+1}^y), \quad (\text{S25})$$

where  $i$  refers to the sites on the chain, and  $J \equiv \cos \xi$ ,  $K \equiv \sin \xi$  with  $\pi < \xi < 3\pi/2$ . The second term in Eq. (S25) corresponds to alternating  $x-x$  and  $y-y$  Kitaev couplings. The Kitaev term breaks continuous spin-rotation symmetry, leaving only discrete symmetries, such as a  $\pi/2$  spin rotation about  $\hat{z}$  axis combined with unit lattice translation. Classical ground states are accidentally degenerate ferromagnetic

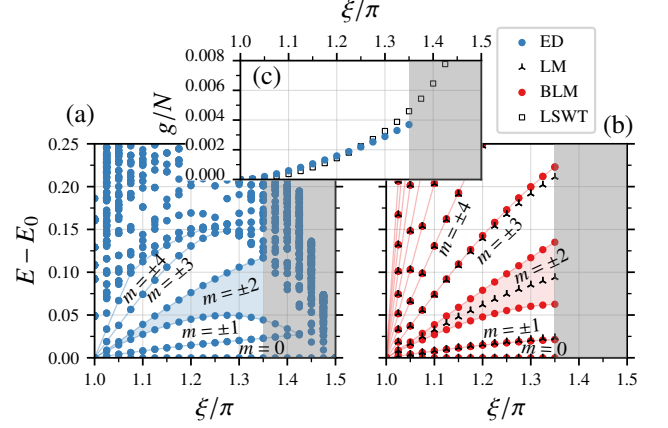

FIG. S3. Ferromagnetic Heisenberg-Kitaev spin chain of  $N = 20$  sites with periodic boundary conditions. (a) Low-energy ED spectrum. (b) The LM and BLM model spectra. The  $g$  value for the BLM model is determined from the splitting in the ED spectrum. (c) Comparison of  $g$  obtained from LSWT and splitting in the ED spectrum. Grey-shaded regions in all panels indicate the regime where the low-energy physics deviates from the BLM description as it approaches a different phase in  $1.44\pi \lesssim \xi \lesssim 1.5\pi$  [16].

configurations pointing along any arbitrary direction in the  $\hat{x} - \hat{y}$  plane, with ObQD selecting only those aligned along  $\pm \hat{x}, \pm \hat{y}$  directions. This is confirmed by analyzing the properties of the ground state using density matrix renormalization group (DMRG) method, although in  $\pi < \xi \lesssim 1.44\pi$  [16]. For  $1.44\pi \lesssim \xi \lesssim 1.5\pi$ , a different phase emerges.

The ED spectrum, obtained using the combined lattice translational and spin-rotational symmetry mentioned above, is presented in Fig. S3(a). To identify the splittings due to ObQD, we next construct the effective description. Using the same projections as those employed for the ferromagnetic Heisenberg-compass model on the square lattice [Sec. II A], and omitting the constant terms, we obtain

$$\mathcal{H}_{\text{LM}} = -\frac{K}{2(N-1)} (S_{\text{tot}}^z)^2. \quad (\text{S26})$$

This Hamiltonian is the same as that for the ferromagnetic Heisenberg-compass model on the square lattice, except the prefactor. Therefore, their spectra are similar, as can be seen in Fig. S3(b). Since the spin-wave ZPE is minimized by ferromagnetic ground states aligned along  $\pm \hat{x}$  and  $\pm \hat{y}$ , it takes the same form,  $-g \cos 4\phi$ , as in the ferromagnetic Heisenberg-compass model. Therefore, following the same reasoning, we obtain the ObQD-induced perturbation term

$$\mathcal{H}_{\text{pert}} = -\frac{g}{2} \frac{(S_{\text{tot}}^+)^4 + (S_{\text{tot}}^-)^4}{[N/2(N/2+1)]^2}. \quad (\text{S27})$$

This perturbation splits the  $m = \pm 2$  states at first order in perturbation theory, and comparing this with the corresponding splitting from the ED spectrum, we can get an estimate of  $g$  from ED following the steps in Sec. II A as

$$g = \frac{N/2(N/2+1)}{(N/2-1)(N/2+2)} \Delta_{\text{ED}}. \quad (\text{S28})$$

The  $g$  value obtained from the ED data agrees quite well with the value derived from LSWT, as shown in Fig. S3(c). Comparing the BLM spectrum with the values of  $g$  found from ED [Fig. S3(b)] with the low-energy ED spectrum shown in Fig. S3(a) yields good qualitative agreement. Significant disagreement near  $\xi \sim 3\pi/2$  arises due to the existence of a different phase in  $1.44\pi \lesssim \xi \lesssim 1.5\pi$  [16], making the effective

description inapplicable. While the agreement between ED and the effective model spectra is qualitatively good in this one-dimensional example, it is not as good as in the two- and three-dimensional cases. This is likely due to the enhanced quantum fluctuations that are intrinsic to one-dimensional systems, in contrast to their higher-dimensional counterparts.

- 
- [1] E. Lieb and D. Mattis, Ordering energy levels of interacting spin systems, *Journal of Mathematical Physics* **3**, 749 (1962).
  - [2] C. Lhuillier, Frustrated quantum magnets (2005), [arXiv:cond-mat/0502464](#) [cond-mat.str-el].
  - [3] A. Wietek, M. Schuler, and A. M. Läuchli, Studying continuous symmetry breaking using energy level spectroscopy (2017), [arXiv:1704.08622](#) [cond-mat.str-el].
  - [4] N.-G. Zhang, C. L. Henley, C. Rischel, and K. Lefmann, Effective Hamiltonian and low-lying eigenenergy clustering patterns of four-sublattice antiferromagnets, *Phys. Rev. B* **65**, 064427 (2002).
  - [5] T. Roscilde, T. Comparin, and F. Mezzacapo, Rotor/spin-wave theory for quantum spin models with  $u(1)$  symmetry, *Phys. Rev. B* **108**, 155130 (2023).
  - [6] S. Khatua, R. Shankar, and R. Ganesh, Quantum spin quadrumer, *Phys. Rev. B* **97**, 054403 (2018).
  - [7] S. Khatua, D. Sen, and R. Ganesh, Effective theories for quantum spin clusters: Geometric phases and state selection by singularity, *Phys. Rev. B* **100**, 134411 (2019).
  - [8] S. Khatua, S. Srinivasan, and R. Ganesh, State selection in frustrated magnets, *Phys. Rev. B* **103**, 174412 (2021).
  - [9] S. Khatua and R. Ganesh, Berry phase in the rigid rotor: Emergent physics of odd antiferromagnets, *Phys. Rev. B* **105**, 184401 (2022).
  - [10] S. Khatua, G. C. Howson, M. J. P. Gingras, and J. G. Rau, Ground state properties of the Heisenberg-compass model on the square lattice, *Phys. Rev. B* **110**, 104426 (2024).
  - [11] E. Livioti, S. Carretta, and G. Amoretti, S-mixing contributions to the high-order anisotropy terms in the effective spin Hamiltonian for magnetic clusters, *The Journal of Chemical Physics* **117**, 3361 (2002).
  - [12] J. G. Rau, P. A. McClarty, and R. Moessner, Pseudo-Goldstone gaps and order-by-quantum disorder in frustrated magnets, *Phys. Rev. Lett.* **121**, 237201 (2018).
  - [13] J. Chaloupka, G. Jackeli, and G. Khaliullin, Kitaev-Heisenberg model on a honeycomb lattice: Possible exotic phases in iridium oxides  $A_2IrO_3$ , *Phys. Rev. Lett.* **105**, 027204 (2010).
  - [14] J. Chaloupka, G. Jackeli, and G. Khaliullin, Zigzag magnetic order in the iridium oxide  $Na_2IrO_3$ , *Phys. Rev. Lett.* **110**, 097204 (2013).
  - [15] P. Fazekas, *Lecture Notes on Electron Correlation and Magnetism* (World Scientific, New Jersey, 1999).
  - [16] W. Yang, C. Xu, S. Ma, A. Nocera, and I. Affleck, Left-left-right-right magnetic order in spin- $\frac{1}{2}$  Kitaev-Heisenberg chain, *Phys. Rev. B* **112**, 035104 (2025).
  - [17] C. E. Agrapides, J. van den Brink, and S. Nishimoto, Ordered states in the Kitaev-Heisenberg model: From 1D chains to 2D honeycomb, *Scientific Reports* **8**, 1815 (2018).
  - [18] W. Yang, A. Nocera, and I. Affleck, Comprehensive study of the phase diagram of the spin- $\frac{1}{2}$  Kitaev-Heisenberg-Gamma chain, *Phys. Rev. Res.* **2**, 033268 (2020).
  - [19] A. Kitaev, Anyons in an exactly solved model and beyond, *Annals of Physics* **321**, 2 (2006).
